# Supplementary material for: InternVL3: Exploring Advanced Training and Test-Time Recipes for Open-Source Multimodal Models
Source: arXiv:2504.10479 source file (2025-04-19)
Supplement: Supplementary file 2 [file alignment_appendix.tex]

\begin{figure*}[!ht] \label{appendix_alpacaeval}
\vspace{-5mm}
\begin{AIbox}{Prompt in AlpacaEval}
% {\color{blue}\bf Prompt:} \\
% {
%     \textbf{Question:} 
%     Let $R$ be a ring and let $U$ and $V$ be (two-sided) ideals of $R$. Which of the following must also be ideals of $R$?   
   
% }

% \textbf{Error Analysis:} \\
% In crafting its response, the model fails to accurately grasp the concept of an ideal within a ring.
{\color{blue}\bf System Prompt:}\\
You are a highly efficient assistant, who evaluates and selects the best large language model (LLMs) based on the quality of their responses to a given instruction. This process will be used to create a leaderboard reflecting the most accurate and human-preferred answers. \\

{\color{blue}\bf User Prompt:} \\
I require a leaderboard for various large language models. I'll provide you with prompts given to these models and their corresponding outputs. Your task is to assess these responses, and select the model that produces the best output from a human perspective.\\

\textbf{Instruction}
\lstset{style=prompt_json}
\begin{lstlisting}
{
    "instruction": """{instruction}"""
}
\end{lstlisting}

\textbf{Model Outputs}

Here are the unordered outputs from the models. Each output is associated with a specific model, identified by a unique model identifier.\\
\begin{lstlisting}
{
    {
        "model_identifier": "m",
        "output": """{output_1}"""
    },
    {
        "model_identifier": "M",
        "output": """{output_2}"""
    }
}
\end{lstlisting}
\textbf{Task}

Evaluate the models based on the quality and relevance of their outputs, and select the model that generated the best output. Answer by providing the model identifier of the best model. We will use your output as the name of the best model, so make sure your output only contains one of the following model identifiers and nothing else (no quotes, no spaces, no new lines, ...): m or M.\\

\textbf{Best Model Identifier}

\end{AIbox} 
\caption{Prompt used in AlpacaEval}
\label{fig:prompt_of_alpacaeval}
\end{figure*}

\begin{figure*}[!ht] 
\vspace{-5mm}
\begin{AIbox}{Prompt in MTBench}
{\color{blue}\bf System Prompt:}\\
Please act as an impartial judge and evaluate the quality of the response provided by an AI assistant to the user question displayed below. Your evaluation should consider factors such as the helpfulness, relevance, accuracy, depth, creativity, and level of detail of the response. You evaluation should focus on the assistant's answer to the second user question. Begin your evaluation by providing a short explanation. Be as objective as possible. After providing your explanation, you must rate the response on a scale of 1 to 10 by strictly following this format: \textbf{[[rating]]}, for example: \textbf{Rating: [[5]]} \\
{\color{blue}\bf User Prompt:} \\
\lstset{style=prompt_json}
\begin{lstlisting}
<|The Start of Assistant A's Conversation with User|>

### User:
{question_1}

### Assistant A:
{answer_1}

### User:
{question_2}

### Assistant A:
{answer_2}

<|The End of Assistant A's Conversation with User|>
\end{lstlisting}
\end{AIbox} 
\caption{Prompt used in MTBench}
\label{fig:prompt_of_MTBench}
\end{figure*}

% \begin{lstlisting}[style=code]
% # Detect corners using Shi-Tomasi corner detector
% corners = cv2.goodFeaturesToTrack(equalized_image, 
%                                   maxCorners=max_corners, 
%                                   qualityLevel=quality_level, 
%                                   minDistance=min_distance, 
%                                   blockSize=block_size)
% # Mark the corners with circles on the image
% marked_image = equalized_image.copy()
% for corner in corners:
%     x, y = corner.ravel()
%     cv2.circle(marked_image, (int(x), int(y)), 5, (255, 0, 0), -1)  # Draw a blue filled circle at each corner

% # Show the marked image
% plt.imshow(marked_image, cmap='gray')
% plt.axis('off')  # Turn off axis numbers and ticks
% plt.show()

% \end{lstlisting}
